# Supplementary material for: Cross-Domain Object Detection Using Unsupervised Image Translation
Source: arXiv:2601.11779 source file (2026-01-16)
Supplement: Supplementary file 1 [file supplementary_material.tex]

\documentclass[preprint]{elsarticle}
\usepackage{hyperref}
% \modulolinenumbers[1]

\journal{Expert Systems with Applications}
\date{June 1, 2021} 

% my includes
%\usepackage[numbers]{natbib}
%\usepackage{cite}
\usepackage{hyphenat}
\usepackage[cmex10]{amsmath}
\usepackage{amsfonts}
\usepackage{capt-of}% or \usepackage{caption}
\usepackage{xcolor}
\usepackage{xspace}
\usepackage{soul}
\usepackage{diagbox}
\usepackage{multirow}
\setstcolor{red}
\usepackage[shortcuts]{extdash}
% The px template was: \usepackage{subfig}
% But I prefer subcaption, problem?
\usepackage{subcaption}

\usepackage{booktabs}
\usepackage{multirow}
\usepackage{adjustbox}

\usepackage{pifont}% http://ctan.org/pkg/pifont
\newcommand{\cmark}{\ding{51}}%
\newcommand{\ccmark}{\ding{51}{\small\kern-0.7em\ding{55}}}%
\newcommand\doublecheckmark{\checkmark\kern-0.6em\checkmark}

\graphicspath{{figs/}}

%%%%%%%%%%%%%%%%%%%%%%%
%% Elsevier bibliography styles
%%%%%%%%%%%%%%%%%%%%%%%
%% To change the style, put a % in front of the second line of the current style and
%% remove the % from the second line of the style you would like to use.
%%%%%%%%%%%%%%%%%%%%%%%

%% Numbered
%\bibliographystyle{model1-num-names}

%% Numbered without titles
%\bibliographystyle{model1a-num-names}

%% Harvard
%\bibliographystyle{model2-names.bst}\biboptions{authoryear}

%% Vancouver numbered
%\usepackage{numcompress}\bibliographystyle{model3-num-names}

%% Vancouver name/year
%\usepackage{numcompress}\bibliographystyle{model4-names}\biboptions{authoryear}

%% APA style
%\bibliographystyle{model5-names}\biboptions{authoryear}

%% AMA style
%\usepackage{numcompress}\bibliographystyle{model6-num-names}

\pdfstringdefDisableCommands{%
  \def\corref#1{<#1>}%
}

%% `Elsevier LaTeX' style
% \bibliographystyle{elsarticle-num}
\bibliographystyle{model5-names}\biboptions{authoryear}
%%%%%%%%%%%%%%%%%%%%%%%

\makeatletter
  \long\def\pprintMaketitle{\clearpage
  \iflongmktitle\if@twocolumn\let\columnwidth=\textwidth\fi\fi
  \resetTitleCounters
  \def\baselinestretch{1}%
  \printFirstPageNotes
  \begin{center}%
 \thispagestyle{pprintTitle}%
   \def\baselinestretch{1}%
    \Large\@title\par\vskip18pt
    \normalsize\elsauthors\par\vskip10pt
    \footnotesize\itshape\elsaddress\par\vskip36pt
    % \hrule\vskip12pt
    % \ifvoid\absbox\else\unvbox\absbox\par\vskip10pt\fi
    % \ifvoid\keybox\else\unvbox\keybox\par\vskip10pt\fi
    % \hrule\vskip12pt
    \end{center}%
  \gdef\thefootnote{\arabic{footnote}}%
  }
\makeatother

\begin{document}

\begin{frontmatter}
\title{Supplementary Material\\Cross-Domain Object Detection Using\\Unsupervised Image Translation}

\author[ufes]{Vinicius F. Arruda\corref{mycorrespondingauthor}}
\cortext[mycorrespondingauthor]{Corresponding author}
\ead{viniciusferracoarruda@gmail.com}

\author[ufes]{Rodrigo F. Berriel}
% \ead{rfberriel@inf.ufes.br}

\author[ufes,ifes]{Thiago M. Paix\~ao}
% \ead{paixao@gmail.com}

\author[ufes]{\\Claudine Badue}
% \ead{claudine@lcad.inf.ufes.br}

\author[ufes]{Alberto F. De Souza}
% \ead{alberto@lcad.inf.ufes.br}

\author[unitn]{Nicu Sebe}
% \ead{sebe@disi.unitn.it}

\author[ufes]{Thiago Oliveira-Santos}
% \ead{todsantos@lcad.inf.ufes.br}

\address[ufes]{Universidade Federal do Esp\'irito Santo (UFES), Brazil}
\address[ifes]{Instituto Federal do Esp\'irito Santo (IFES), Brazil}
\address[unitn]{University of Trento (UNITN), Italy}

\end{frontmatter}

% \linenumbers

\section{Results}
\subsection{Learning from synthetic data}

In \autoref{tab:results-synthetic-full} and \autoref{fig:results-synthetic-full} are shown additional results and translation samples from Sim10k to Cityscapes. In general, the addition of source data in the training process did not increase the mAP significantly.

\begin{table}[ht!]
    \centering
    % \begin{adjustbox}{width=0.65\columnwidth,center}
    \begin{tabular}{c | c c | c c | c} 
     \toprule
      & \multicolumn{2}{c}{Real} & \multicolumn{2}{|c|}{Fake} & \\
     Method & S & T & C & A & car AP\\
     \midrule\midrule
     Source-only & \cmark & & & & 34.7 \\ 
     \hline
     DA-Faster \cite{dafaster} & \cmark & \ccmark & & & 27.3 \\
     Strong-Weak DA \cite{strongweakda} & \cmark & \ccmark & & & 31.7 \\
     \hline
    OURS-C & & & \cmark & & 42.4 \\
    OURS-A & & & & \cmark & 43.7 \\
    OURS-C+A  & & & \cmark & \cmark & \textbf{44.6} \\
    OURS-S+C  & \cmark & & \cmark & & 42.6 \\
    OURS-S+A  & \cmark & & & \cmark & 44.5 \\
    OURS-S+C+A  & \cmark & & \cmark & \cmark & \textbf{44.6} \\
     \hline
     Target-only & & \cmark & & & 58.9 \\
    %  \hline
    %  Upper-bound \doublecheckmark & \doublecheckmark & & & & 6344 \\
     \bottomrule
    \end{tabular}
    % \end{adjustbox}
    \caption{Sim10k$\rightarrow$Cityscapes: Results from training with annotated Sim10k (S) and nonannotated Cityscapes (T), evaluating on Cityscapes. The check-mark denotes which data was used during training, and if crossed, only non-annotated data was used. Fake data was acquired by translating Sim10k using CycleGAN (C) and AST-AdaIN (A).}
    \label{tab:results-synthetic-full}
\end{table}

\begin{figure}[ht!]
	\centering
	\begin{subfigure}{\linewidth}
	    \centering
	    \includegraphics[width=\textwidth]{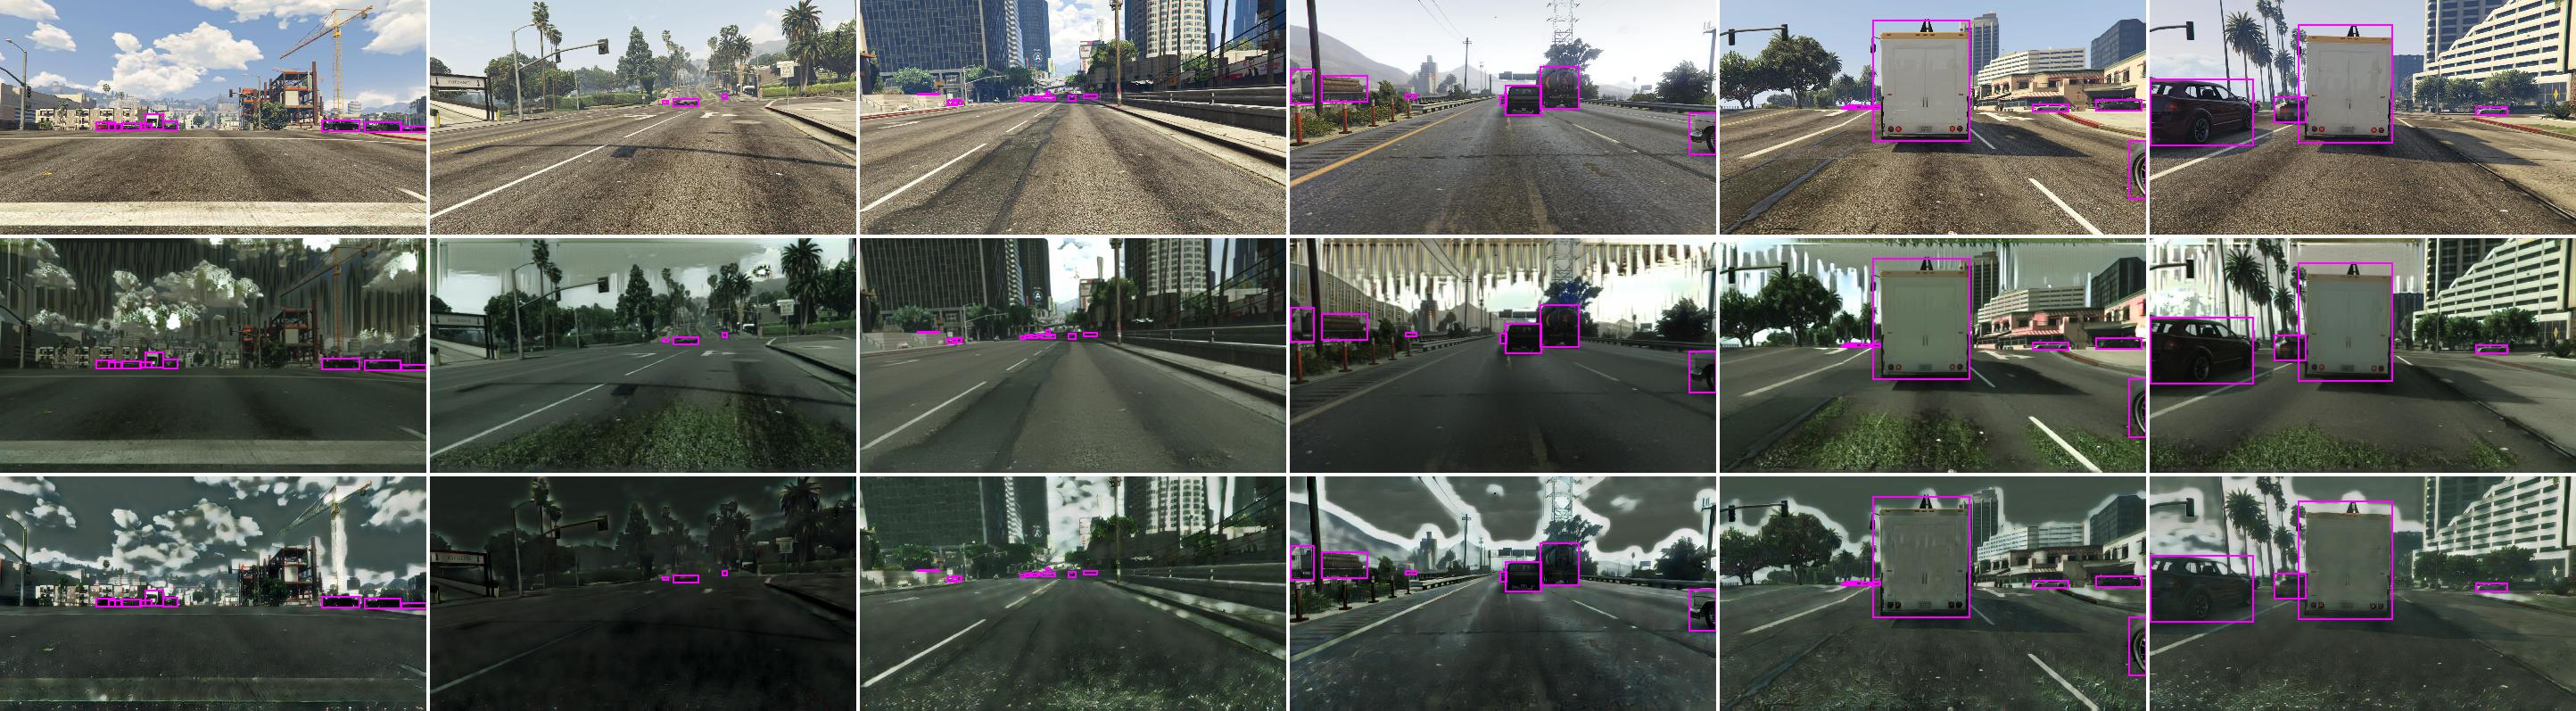}
	\end{subfigure}
	\caption{Samples of translated images with their respective bounding boxes. The real source training images are shown in the first row and their respective fake-target versions are shown in the second and third row for the CycleGAN and AST-AdaIN models, respectively.}
	\label{fig:results-synthetic-full}
\end{figure}

\subsection{Driving in adverse weather}
In Tables \ref{tab:results-weather-target-full1} and \ref{tab:results-weather-target-full2} are shown additional and detailed results from the Cityscapes to Foggy-Cityscapes datasets. \autoref{fig:results-weather-target-full} depicts more translation samples.

\begin{table}[ht!]
    % \centering
    \begin{adjustbox}{width=\columnwidth,center}
    \begin{tabular}{c | c c | c c | c c c c c c c c | c} 
     \toprule
      & \multicolumn{2}{c}{Real} & \multicolumn{2}{|c}{Fake} & \multicolumn{8}{|c|}{AP} & \multirow{2}{*}{mAP}\\
     Method & S & T & C & A & person & rider & car & truck & bus & train & mcycle & bicycle & \\
     \midrule\midrule
     Source-only & \cmark & & & & 28.9 & 40.5 & 36.1 & 18.1 & 27.5 & 10.0 & 22.8 & 32.9 & 27.1 \\ 
     DA-Faster \cite{dafaster} & \cmark & \ccmark & & & 28.5 & 42.0 & 42.6 & 21.8 & 43.9 & 28.9 & 22.0 & 35.2 & 33.1 \\
     Strong-Weak DA \cite{strongweakda} & \cmark & \ccmark & & & 29.2 & 41.0 & 44.9 & 24.6 & 37.6 & 21.3 & 28.1 & 35.9 & 32.8 \\
     \hline
    OURS-C & & & \cmark & & 32.7 & 44.0 & 52.4 & \textbf{31.2} & 51.5 & 39.9 & 28.6 & 34.5 & 39.4 \\
    OURS-A  & & & & \cmark & 27.9 & 39.9 & 44.5 & 21.1 & 38.5 & 20.5 & 23.2 & 30.6 & 30.8 \\
    OURS-C+A  & & & \cmark & \cmark & 33.1 & 45.4 & 51.8 & 29.2 & 48.4 & 41.4 & 29.9 & 35.8 & 39.5 \\
    OURS-S+C  & \cmark & & \cmark & & \textbf{33.5} & 44.3 & \textbf{53.0} & 30.0 & \textbf{53.0} & \textbf{51.6} & \textbf{30.4} & 36.3 & \textbf{41.5} \\
    OURS-S+A  & \cmark & & & \cmark & 31.1 & 44.5 & 47.4 & 24.2 & 40.2 & 35.0 & 29.7 & 33.9 & 35.7 \\
    OURS-S+C+A  & \cmark & & \cmark & \cmark & 34.4 & \textbf{45.6} & 52.9 & 30.1 & 50.1 & 48.8 & 30.3 & \textbf{37.2} & 41.2 \\
     \hline
     Target-only & & \cmark & & & 35.9 & 47.6 & 56.0 & 35.6 & 57.5 & 50.9 & 36.0 & 39.1 & 44.8 \\
     \bottomrule
    \end{tabular}
    \end{adjustbox}
    \caption{Cityscapes$\rightarrow$FoggyCityscapes: Results from training with annotated Cityscapes (S) and non-annotated Foggy Cityscapes (T), evaluating solely on Foggy Cityscapes. The check-mark denotes which data was used during training, and if crossed, only non-annotated data was used. Fake data was acquired by translating Cityscapes using CycleGAN (C) and AST-AdaIN (A).}
    \label{tab:results-weather-target-full1}
\end{table}

\begin{table}[ht!]
    % \centering
    \begin{adjustbox}{width=\columnwidth,center}
    \begin{tabular}{c | c c | c c | c c c c c c c c | c} 
     \toprule
      & \multicolumn{2}{c}{Real} & \multicolumn{2}{|c}{Fake} & \multicolumn{8}{|c|}{AP} & \multirow{2}{*}{mAP}\\
     Method & S & T & C & A & person & rider & car & truck & bus & train & mcycle & bicycle & \\
     \midrule\midrule
     Source-only & \cmark & & & &33.6 & 45.0 & 47.1 & 26.5 & 44.8 & 26.1 & 31.1 & 36.5 & 36.3 \\ 
     DA-Faster \cite{dafaster} & \cmark & \ccmark & & & 31.1 & 44.3 & 47.7 & 28.0 & 51.3 & 33.9 & 28.9 & 36.5 & 37.7 \\
     Strong-Weak DA \cite{strongweakda} & \cmark & \ccmark & & & 33.4 & 45.3 & 50.6 & 29.9 & 49.4 & 32.5 & 33.2 & 39.2 & 39.2 \\
     \hline
    OURS-C & & & \cmark & & 33.0 & 43.2 & 53.8 & 31.7 & 53.4 & 36.3 & 31.4 & 34.3 & 39.6 \\
    OURS-A & & & & \cmark & 31.5 & 42.8 & 50.4 & 28.3 & 48.9 & 27.2 & 26.2 & 33.5 & 36.1 \\
    OURS-C+A & & & \cmark & \cmark & 34.3 & 46.3 & 54.7 & 33.0 & 53.1 & 39.7 & 33.2 & 37.6 & 41.5 \\
    OURS-S+C & \cmark & & \cmark & & 35.9 & 47.1 & \textbf{56.3} & 34.7 & \textbf{58.1} & 50.5 & \textbf{36.1} & 38.5 & 44.6 \\
    OURS-S+A & \cmark & & & \cmark & 34.5 & 47.1 & 52.7 & 32.9 & 51.1 & 37.0 & 34.7 & 36.7 & 40.8 \\
    OURS-S+C+A  & \cmark & & \cmark & \cmark & \textbf{36.1} & \textbf{48.0} & 55.6 & \textbf{35.6} & 57.7 & \textbf{52.5} & 35.2 & \textbf{38.8} & \textbf{44.9} \\
     \hline
     Target-only & \cmark & \cmark & & & 37.5 & 50.1 & 57.5 & 35.9 & 59.1 & 48.7 & 39.7 & 41.8 & 46.3 \\
     \bottomrule
    \end{tabular}
    \end{adjustbox}
    \caption{Cityscapes$\rightarrow$FoggyCityscapes: Results from training with annotated Cityscapes (S) and non-annotated Foggy Cityscapes (T), evaluating on both source and target dataset. The check-mark denotes which data was used during training, and if crossed, only non-annotated data was used. Fake data was acquired by translating Cityscapes using CycleGAN (C) and AST-AdaIN (A).}
    \label{tab:results-weather-target-full2}
\end{table}

\begin{figure}[ht!]
	\centering
	\begin{subfigure}{\linewidth}
	    \centering
	    \includegraphics[width=\textwidth]{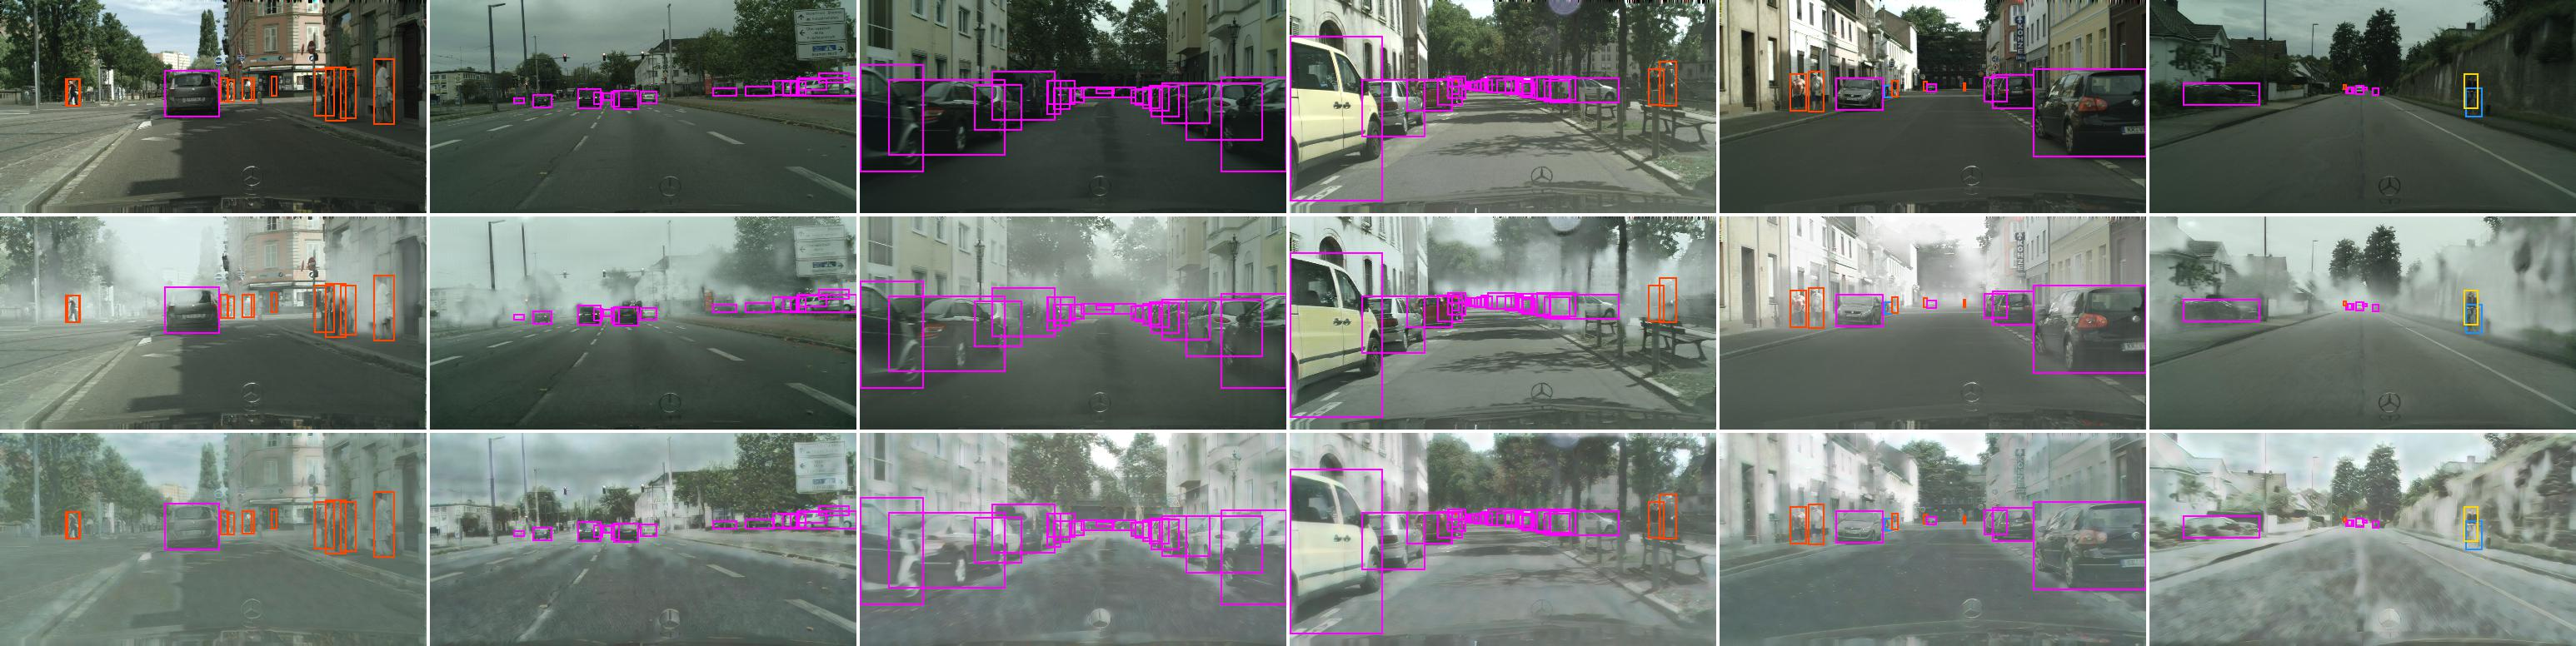}
	\end{subfigure}
	\caption{Samples of translated images with their respective bounding boxes. The real source training images are shown in the first row and their respective fake-target versions are shown in the second and third row for the CycleGAN and AST-AdaIN models, respectively.}
	\label{fig:results-weather-target-full}
\end{figure}

\subsection{Cross-camera adaptation}
Full results are shown in \autoref{tab:results-city-kitti-full} and additional translation samples are shown in \autoref{fig:results-city-kitti-full}.

% Full table results cross camera
\begin{table}[ht!]
    % \centering
    \begin{adjustbox}{width=\columnwidth,center}
    \begin{tabular}{c | c c | c c | c c | c c | c c | c c} 
     \toprule
      & & & & & \multicolumn{4}{c}{car AP (C$\rightarrow$ K)} & \multicolumn{4}{|c}{car AP (K$\rightarrow$ C)}\\
      & \multicolumn{2}{c}{Real} & \multicolumn{2}{|c|}{Fake} & \multicolumn{2}{c|}{Protocol 1} & \multicolumn{2}{c}{Protocol 2} & \multicolumn{2}{|c|}{Protocol 1} & \multicolumn{2}{c}{Protocol 2}\\
     Method & S & T & C & A & T & S+T & T & S+T & T & S+T & T & S+T \\
     \midrule\midrule
     Source-only & \cmark & & & & 74.3 & 71.9 & 74.1 & 68.2 & 29.1 & 80.0 & 28.6 & 65.2\\
     \hline
     DA-Faster \cite{dafaster} & \cmark & \ccmark & & & 71.3 & 68.8 & 70.5 & 64.5 & 31.8 & 81.2 & 30.6 & 66.5\\
     Strong-Weak DA \cite{strongweakda} & \cmark & \ccmark & & & 64.3 & 63.2 & 70.1 & 64.9 & 36.1 & \textbf{82.1} & 35.0 & \textbf{68.8}\\
     \hline
    OURS-C & & & \cmark & & 75.0 & 72.0 & 74.8 & 67.1 & 34.9 & 77.0 & 36.0 & 66.2\\
    OURS-A & & & & \cmark & 72.3 & 69.3 & 71.4 & 64.0 & \textbf{38.7} & 78.5 & 36.8 & 66.1\\
    OURS-C+A  & & & \cmark & \cmark & 75.9 & 73.0 & \textbf{76.5} & 69.0 & 34.5 & 79.6 & 35.6 & 67.4\\
    OURS-S+C  & \cmark & & \cmark & & 76.1 & 73.3 & 75.9 & 69.4 & 36.3 & 81.3 & \textbf{36.9} & 68.5\\
    OURS-S+A & \cmark & & & \cmark & 75.4 & 72.9 & 74.9 & 68.8 & 35.1 & 80.6 & 35.7 & 68.0\\
    OURS-S+C+A & \cmark & & \cmark & \cmark & \textbf{76.3} & \textbf{73.7} & \textbf{76.5} & \textbf{70.1} & 36.7 & 80.8 & 35.5 & 68.3\\
     \hline
     \multirow{2}{*}{Target-only} & & \cmark & & & 88.2 & - & 84.9 & - & 58.9 & - & 58.9 & -\\
      & \cmark & \cmark & & & - & 86.1 & - & 78.3 & - & 86.1 & - & 78.3\\
     \bottomrule
    \end{tabular}
    \end{adjustbox}
    \caption{Cityscapes$\rightarrow$KITTI (C$\rightarrow$K): Results from training with annotated Cityscapes
    (S) and non-annotated KITTI (T), evaluating solely on KITTI (T) or on both (S+T). KITTI$\rightarrow$Cityscapes (K$\rightarrow$C): Results from training with annotated KITTI (S) and nonannotated Cityscapes (T), evaluating solely on Cityscapes (T) or on both (S+T). The checkmark denotes which data was used during training, and if crossed, only non-annotated data was used. Fake data was acquired by translating the source training set using CycleGAN (C) and AST-AdaIN (A).}
    \label{tab:results-city-kitti-full}
\end{table}

\begin{figure}[ht!]
	\centering
	\begin{subfigure}{\linewidth}
	    \centering
	    \includegraphics[width=\textwidth]{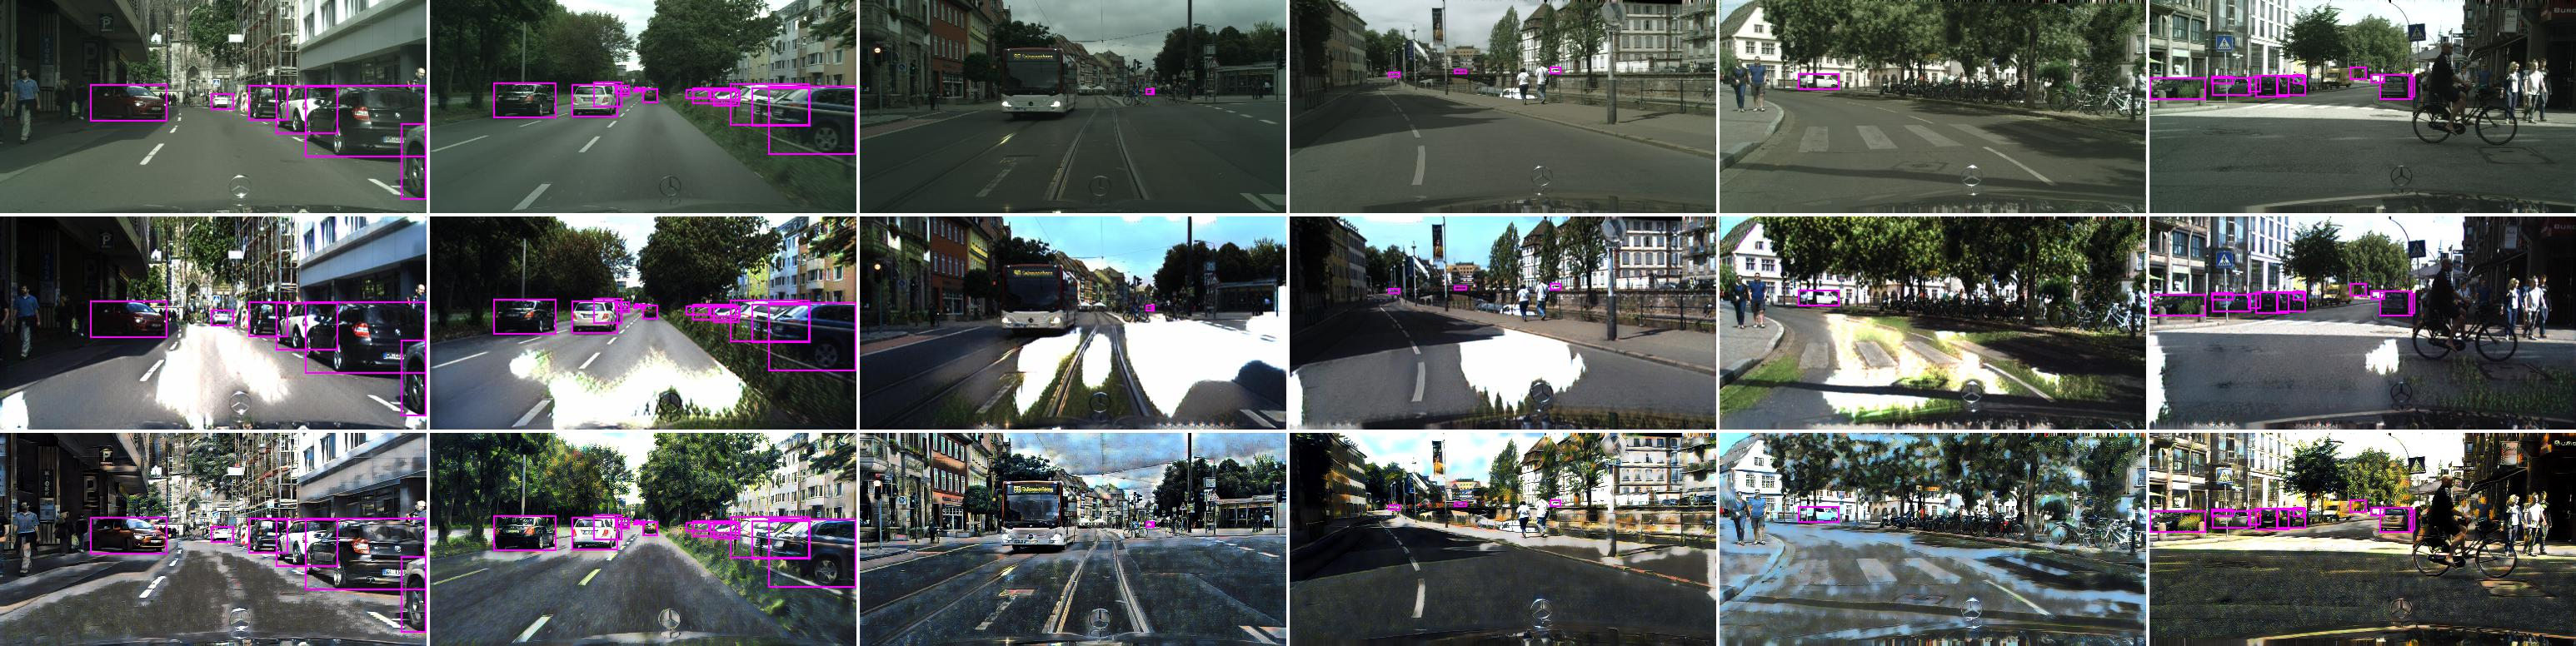}
	    \includegraphics[width=\textwidth]{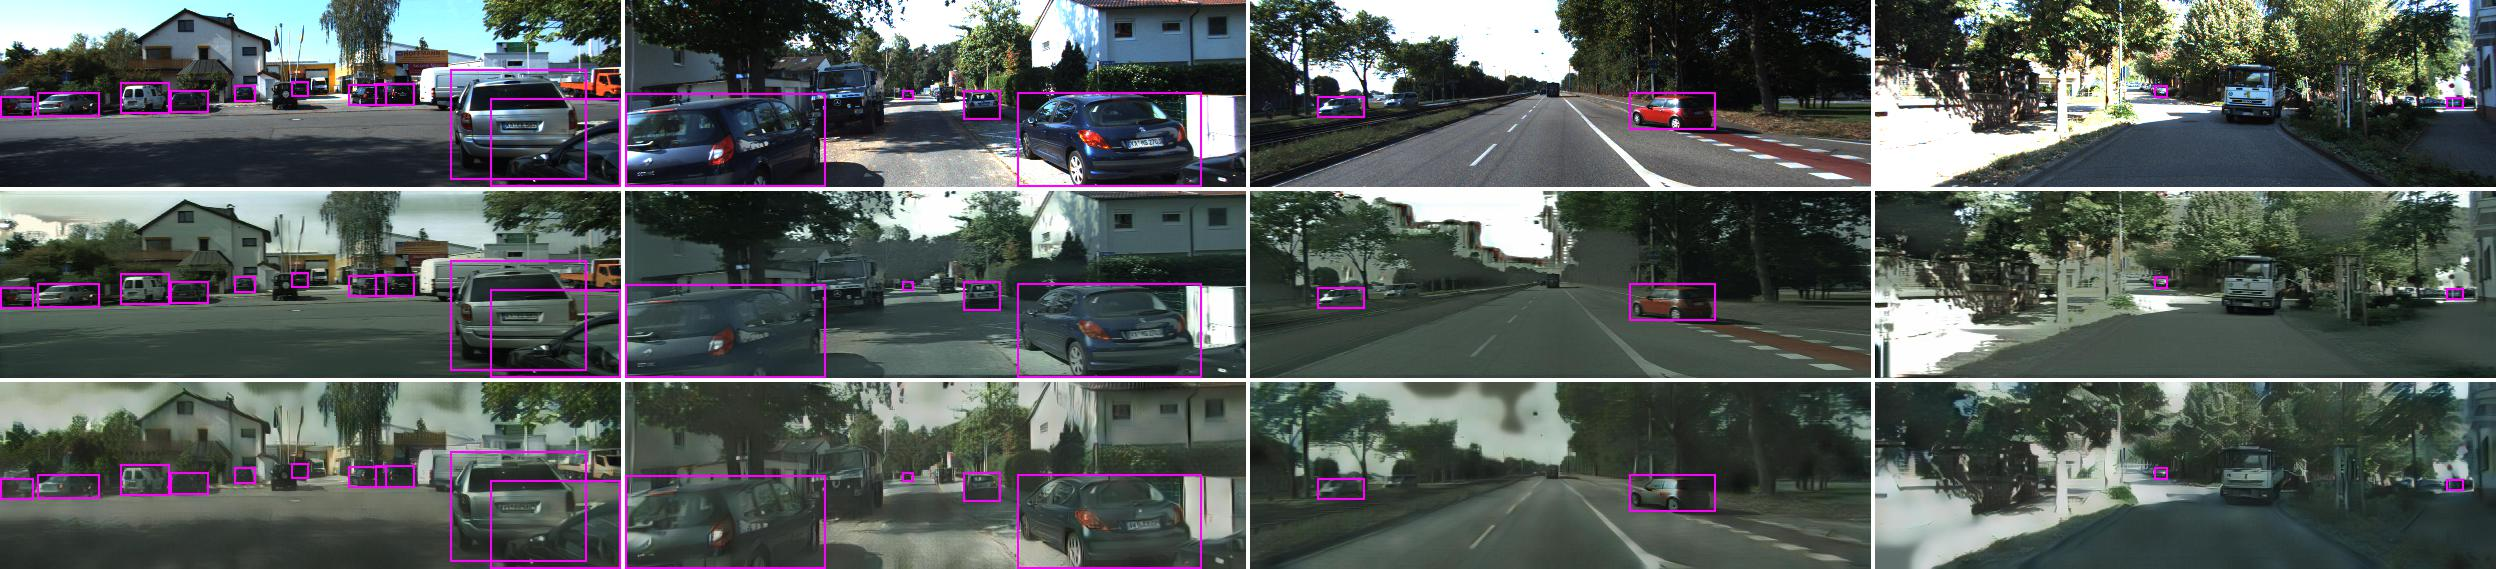}
	\end{subfigure}
	\caption{Samples of translated images with their respective bounding boxes. Top: the translation from Cityscapes to KITTI, and vice-versa for the bottom one. The real source training images are shown in the first row and their respective fake-target versions are shown in the second and third row for the CycleGAN and AST-AdaIN models, respectively.}
	\label{fig:results-city-kitti-full}
\end{figure}

To support the use of the latest metric version (Pascal VOC 2012), we evaluated the scenario using the fake data from CycleGAN on the target domain using the previous metric version (Pascal VOC 2007), achieving $40.3\%$ in mAP (in contrast to $39.4\%$). For the state-of-the-art works, evaluating on the same domain with the previous metric version, the mAP for DA-Faster and Strong-Weak DA was $27.6\%$ and $34.3\%$ (in contrast to $33.1\%$ and $32.8\%$), respectively.

\biboptions{sort&compress}
\bibliography{sup_refs}

\end{document}
